# Supplementary material for: Scaling Up to Excellence: Practicing Model Scaling for Photo-Realistic Image Restoration In the Wild
Source: arXiv:2401.13627 source file (2024-04-03)
Supplement: Supplementary file 1 [file direct1024.tex]

%%%%%%%%%%%%%%%%%%%%%%%%%%%%%%%%%%%%%%%%%%%%%%%%%%

\begin{figure*}[t]
	%\newlength-4mm
	%\setlength{-4mm}{-0.4cm}
	\scriptsize
	\centering
    \vspace{-2mm}
    \includegraphics[width=0.8\linewidth]{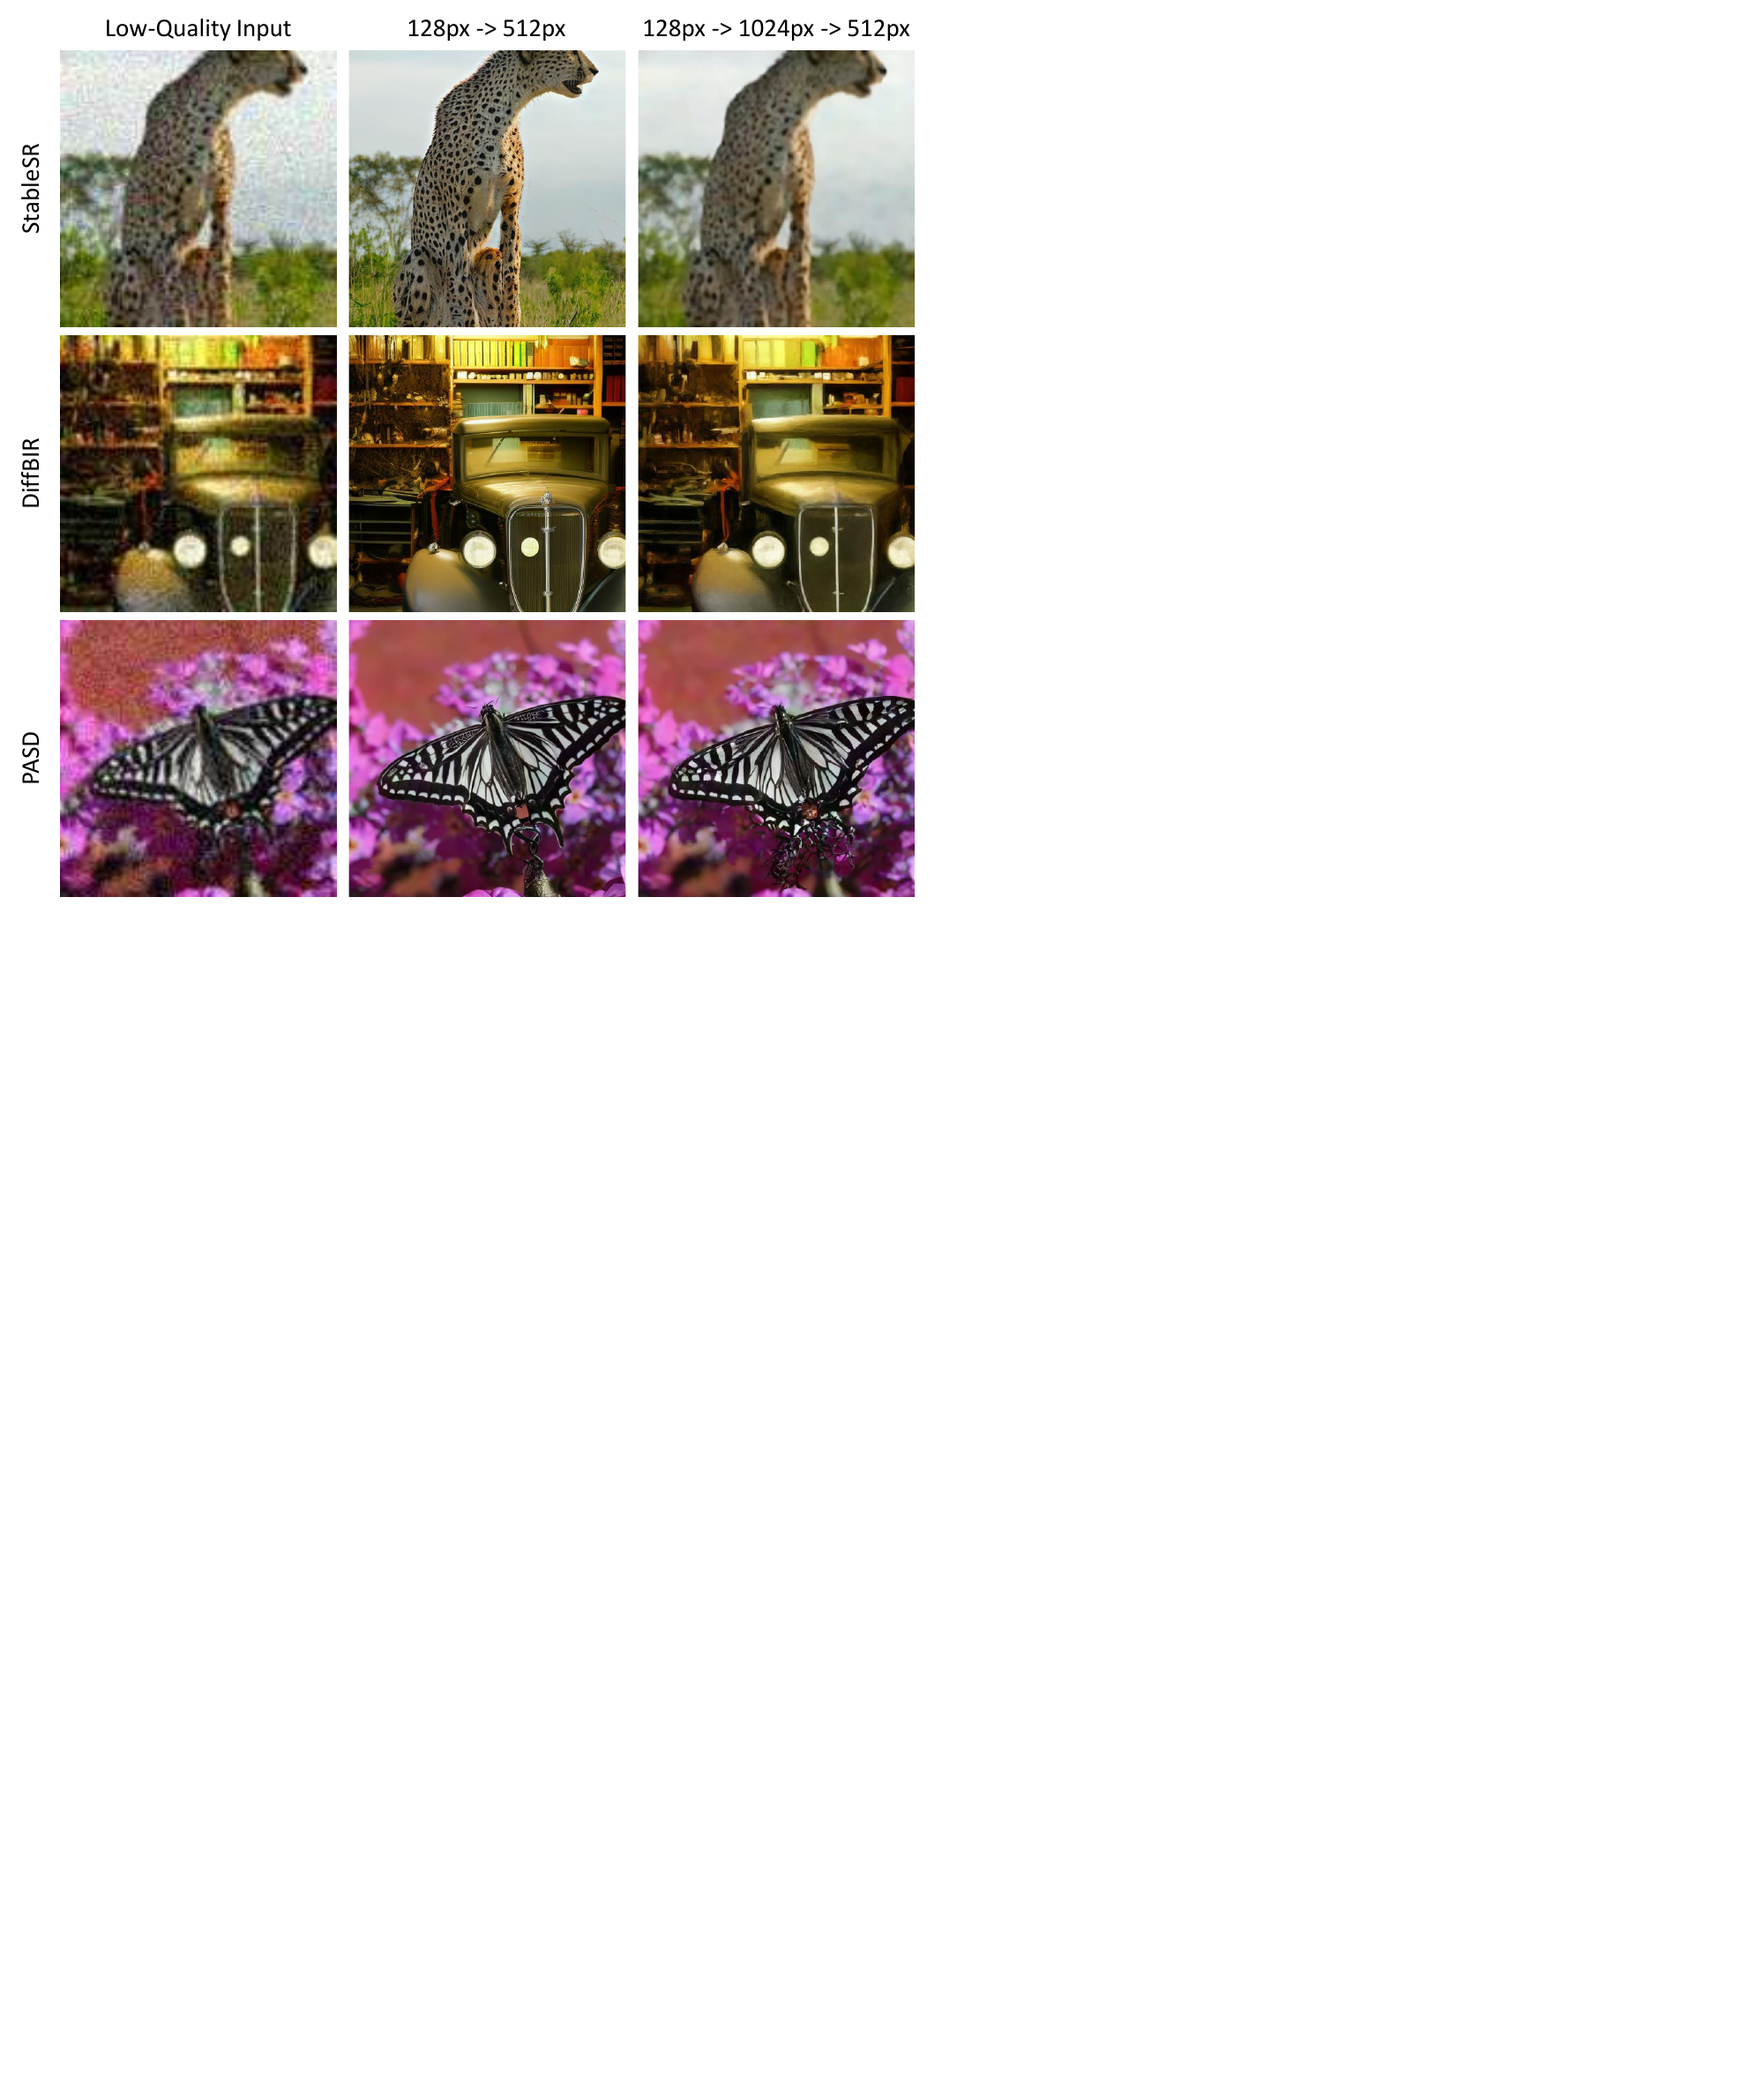}
	% \vspace{-6mm}
	\caption{For restoration models not based on SDXL, employing a larger patch size of $128 \times 128$ leads to suboptimal performance.}
    \label{fig:supp_direct1024}
	% \vspace{-8mm}
\end{figure*}

%%%%%%%%%%%%%%%%%%%%%%%%%%%%%%%%%%%%%%%%%%%%%%%%%%
